# Supplementary material for: maze: Heterogeneous Ligand Unbinding along Transient Protein Tunnels
Source: arXiv:1904.03929 ancillary file (2019-12-16)
Supplement: Supplementary file 1 [file sup.pdf]

# maze: Heterogeneous Ligand Unbinding along Transient Protein Tunnels

**Supporting Information**

Jakub Rydzewski[1, *]

[1]*Institute of Physics, Faculty of Physics, Astronomy and Informatics, Nicolaus Copernicus University, Grudziadzka 5, 87-100 Torun, Poland*

## CONTENTS

I. Benchmark Model Files 1

II. Github Repository 1

III. Version 1

IV. License 1

V. Web Page 2

VI. Chat on Gitter 2

References 2

## I. BENCHMARK MODEL FILES

All necessary files to run a benzene unbinding simulation from T4L were uploaded on a Github repository (https://github/maze-code/benchmark). A `maze` simulation can be run by providing a Plumed input file with the `-plumed plumed.dat` to a standard way of running Gromacs simulations via `mdrun`.

## II. GITHUB REPOSITORY

The implementation is accessible via its Github repository at https://github.com/maze-code/plumed2-maze along Plumed 2.5. The source files of `maze` can be found in `src/maze`. Apart of the current development repository, this version of `maze` will be provided with the official Plumed 2.6 release soon.

## III. VERSION

This `maze` implementation is released as version 1.0.

## IV. LICENSE

The `maze` module is free software: you can redistribute it and/or modify it under the terms of the GNU Lesser General Public License as published by the Free Software Foundation, either version 3 of the License, or (at your option) any later version. This program is distributed in the hope that it will be useful, but without any warranty; without even the implied warranty of merchantability or fitness for a particular purpose. See the GNU Lesser General

Public License for more details. You should have received a copy of the GNU Lesser General Public License along with this program. If not, see http://www.gnu.org/licenses/.

## V. WEB PAGE

Up to date information about the `maze` software (including downloading and installation, citing, materials, and funding) can be obtained from its web page at https://maze-code.github.io. The page is hosted on Github Pages using Jekyll[1] and the `minimal` theme supported by Github.

## VI. CHAT ON GITTER

For the users convenience a community named `maze-code` was created at https://gitter.im/maze-code/. Any questions regarding the `maze` module of Plumed 2 should be asked via Gitter or author's e-mail.

* E-mail: jr@fizyka.umk.pl

[1] Page: https://github.com/pages-themes/minimal.
